# Supplementary material for: MegaScale: Scaling Large Language Model Training to More Than 10,000 GPUs
Source: arXiv:2402.15627 source file (2024-02-23)
Supplement: Supplementary file 1 [file appendix.tex]

\section{Appendix}
\label{sec:appendix}
